# Supplementary material for: HyperBlocker: Accelerating Rule-based Blocking in Entity Resolution using GPUs
Source: arXiv:2410.04349 source file (2024-12-13)
Supplement: Supplementary file 1 [file sec-appendix.tex]

%\nobalance
\appendix
\label{sec-appendix}

\section{Notation Table}
We summarize the frequently used notations in Table~\ref{tab:notation}.

\begin{table}[h]
\vspace{-1ex}
    \begin{center}
    \caption{Summary of frequently used notations}
    \vspace{-2ex}
    \centering
    %\scriptsize
    \footnotesize
    \begin{tabular}{cc}\toprule
        \textbf{Notations} &  \textbf{Definition} \\ \midrule
        $R$  & A relation schema $(\eid, A_1, \dotsc, A_n)$  \\
      $D / P  $ & A set of tuples / a partition of $D$ \\ 
      $m$ & The number of data partitions of $D$ \\ 
      $\kw{Ca}(P)$ & A set of potential matches  from $P$ \\  
      $\varphi / \Delta $ & A matching dependency (\MD) / a set of \MDs \\  
      $p / X / \P$ & A predicate / a precondition / all predicates appeared in $\Delta$ \\  
      $h$ and $h(t_1, t_2)$ & \makecell{A valuation of $\varphi: X \ra l$ that instantiates variables  $t$  and $s$ \\ with tuples  $t_1$ and $t_2$;
      $\varphi$ is a witness at $(t_1, t_2)$  if $h \models X$  } \\  
      $\T/N/\rho$ & An execution plan (tree) / a node /  a path of $\T$ \\  
      $e/\kw{score}(e)$ & An edge $(N_1, N_2)$ of $\T$ / the score of $e$ \\  
      %$\P$ &  The set of predicates in $\Delta$ \\\hline
      \makecell{$\kw{cost}(p, D)$  ($\hat{\kw{cost}}(p, D)$)} &  The (estimated) evaluation cost of $p$ on $D$ \\
      %$\N$ &  A shallow feed-forward neural network \\\hline
      $\kw{sp}(p, D)$ &  The probability of $p$ being satisfied on $D$ \\
      $\kw{wp}(p, D)$ &  The probability of $\varphi$ being a witness \\
      $n_t$/$n_w$ &  The size of intervals / the size of window \\
      %$M$ &  The number of GPUs \\\hline
      \bottomrule
    \end{tabular}
    \label{tab:notation}
    \end{center}
\vspace{-3ex}
\end{table}

\section{Training of Shallow Model}
To train $\N$,
we collect training data from historical logs,
where
each training instance is in form $(x, y)$;
here $x$ is triplet  $(p, t_1, t_2)$ and $y$ is its label, \ie the measured time of evaluating $p$ at $(t_1, t_2)$.
We train $\N$ offline, using stochastic gradient descent with the mean square error loss.
While the training time is not our focus,
	$\N$ converges quickly in a few pass~\cite{kraska2018case},
	since it has few parameters.

\section{More Optimizations}
\Hyper is implemented in 4K+ lines of C++/CUDA code \reviseY{with the pipelined architecture. It also offers the following optimizations.}
\looseness=-1

\vspace{-0.6ex}
\subsection{Parallel write conflict}
\label{subsec:conflict}
When thousands of threads on a GPU are executing in parallel, 
each thread may produce an uncertain number of results. 
Therefore, \revise{these}
threads will compete for GPU memory and 
it is hard for them to decide the position \revise{where} they should write the results. 
This is called \emph{parallel write conflict}. %\looseness=-1
Many GPU-based systems,
\eg Pangolin~\cite{Pangolin}, address this by a costly two-round procedure,
\ie they scan the threads twice to (a) record the number of results produced
by each thread and (b) write results. 
%This method, however, leads to a severe performance decline.
Other methods, \eg GSI \cite{GSI},
estimate the maximum size of results of each thread for space pre-allocation,
which, however, leads to low memory utilization. \looseness=-1

To alleviate this, we maintain a local buffer for each TB at shared memory,
so that only threads in this TB will compete for this buffer.
Moreover, the local buffer is divided into two parts.
Initially, all threads in a TB use their
synchronization primitives to compute write offsets and write to
the first part.
When the first part is full,
this TB will compete with other TBs and flush
its buffered results to GPU memory, by 
computing the global offset with an atomic increment operation;
meanwhile, all threads in this TB start to buffer in the second part of the local buffer,
and the cycle repeats. %\looseness=-1

\subsection{Data transfer between host and devices}
\label{subsec:partition}
It is widely recognized that data transfer between CPUs and GPUs is a bottleneck in CPUs/GPUs computation~\cite{GPU-Accelerated-Subgraph-Enumeration}.
Fortunately, the use of CUDA streams allows to conduct data transfer and GPU execution simultaneously,
to ``cancel'' the excessive data shipment cost.
\looseness=-1

\revise{
Recall that relation $D$ is divided into multiple partitions $P_1, \ldots,  \allowbreak  P_m$.
% Thank to many schema-aware data partition methods~\cite{}\tbf, 
% the policy is simple. \kw{HyperBlocker} can firstly group the entities of $\E$ into 
% a number of clusters  $\{E_1, E_2, ...,E_n\}$ by using one of these methods. 
\kw{HyperBlocker} extends~\cite{miniGraph} and iteratively processes partitions in a pipelined manner.}
%extended from~\cite{miniGraph}, .
Specifically, the out-of-device processing of each partition $P$ is 
divided into three steps: 
(1) Read  $P$ into device memory.
(2) Split $P$ into intervals and process each interval.
(3) Write the result $\kw{Ca}(P)$ back to host memory. 
Then
\kw{HyperBlocker} conducts the evaluation on in-device partitions while loading pending ones from and writing results back to
 the host memory. 
\looseness=-1

\reviseX{
\subsection{More choices for parallelism}
There are indeed other design choices for parallelism:

\mbi
\item[(1)] \emph{Rule-level parallelism},
where the entire warp is assigned to each tuple pair and rules
are evaluated in parallel, \ie each thread in the warp is responsible for the evaluation of a rule;
\item[(2)] \emph{Predicate-level parallelism}, where the entire warp is assigned to each tuple pair and rules
are evaluated sequentially.
Within each rule, predicates are evaluated in parallel and
each thread is responsible for evaluating a predicate.
The warp moves to the next rule only after all predicates of the current rule are evaluated. \looseness=-1
\item[(3)] \emph{Token-level parallelism},
that only works for texts. Each text comparison utilizes multiple threads for parallel processing,
\eg each thread compares the equality of a character/token of two texts. \looseness=-1
\mei

However,
for rule-level parallelism,
there can be unnecessary computation,
\eg even a thread finds a witness $\varphi$ at $(t_1, t_2)$,
other threads may be still checking other rules in $\Delta$,
which is not needed,
since one witness suffices to decide  $(t_1, t_2)$ makes a potential match. \looseness=-1

Similarly, in predicate-level parallelism,
even a thread finds a a predicate $p$ in $\varphi$ such that $h(t_1, t_2) \not \models p$,
other threads may still be checking  other predicates in $\varphi$,
which is also not needed,
since $h(t_1, t_2) \not \models p$ suffices to conclude that $\varphi$ is not a witness at $(t_1, t_2)$.
Worse still,
it treats all predicates equally potent for evaluation and may incur additional synchronization cost.
Consider a rule $\varphi: X \ra l$,
where $X$ consists of multiple predicates
and each predicate is evaluated by a thread.
Given a tuple pair $(t_1, t_2)$,
its evaluation times on different predicates can be different.
In other words,
even a thread finds a predicate $p$ in $\varphi$ such that $h(t_1, t_2) \models p$,
it has to wait for results from
other threads to make a final decision,
since $\varphi$ is a witness at $(t_1, t_2)$ only if $h(t_1, t_2)$ satisfies all predicates in $X$.
As evidence, when testing on a dataset with 6M tuple pairs,
tuple-level parallelism is 
 7.3$\times$ faster than predicate-level one.

Token-level parallelism also inherits the synchronization issues 
and worse still,
it only works for textual attributes.
}

\eat{ 
Consider 
(1) \emph{Inter-Rule-Level Parallelism}: 
In this approach, the warp executes an entire set of rules in parallel. The system evaluates all rules simultaneously, each on separate threads of a warp. This method is inefficient due to branch divergence and workload skewness among different rules; 
(2) \emph{Inter-Predicate-Level Parallelism}: the warp executes rules sequentially, but within each rule, the predicates are evaluated in parallel, with each thread corresponding to a predicate.
The warp can move to the next rule only after all predicates of the current rule are completely evaluated. This results in synchronization costs, where threads have to wait for results from other threads, and disrupts the execution plan, causing low-priority predicates to be evaluated (Section~\ref{sec-plan}).
(3) \emph{Intra-Predicate-Level Parallelism}: 
In this approach, the evaluation of predicates within a rule is done sequentially, but each predicate evaluation utilizes multiple threads of a warp for fine-grained parallel processing. For example, for two long texts, a warp of threads can be used to compute their similarity. This method leads to wasted computational power when encountering simpler, integer-based predicates.}

\section{Additional Experiments}
%We experimented with two dataset including $\kw{Songs_{sub}}$, and \kw{TFACC_{large}}, Table~\ref{tab:dataset_new} lists their details. 
Below we report additional experimental results.

\stitle{Comparison with similarity join.}
\reviseY{Recall that \kw{Faiss} often serves as a key component of many ER solutions~\cite{DeepER,DeepBlocking},
we compared \kw{Faiss} with \Hyper as follows.}
We sampled 50,863 tuples from \kw{Songs}, \reviseX{where} \Hyper conducts rule-based blocking  by taking these tuples as a single partition,
while \kw{Faiss} converts each tuple to an embedding using FastText~\cite{fasttext}
and gets its top-$K$ nearest neighbors, varying $K$ from 1 to 100.
As shown in 
Table~\ref{tab:simVsEr},
\Hyper is more accurate and 3.65$\times$ faster than \kw{Faiss} on average. %\looseness=-1

\begin{table}[t]
    \caption{\kw{Faiss} vs. \Hyper}\label{tab:simVsEr}
    \setlength{\tabcolsep}{5pt}
    \vspace{-2ex}
    \begin{minipage}[t]{1\linewidth}
	\centering
  	\scriptsize
		{%\fontsize{6pt}{1em} 
            \selectfont 
			\begin{tabular}{cc cccc}
                \toprule
                
                %\multirow{2}{*}{\textbf{Method}} & \multirow{2}{*}{\textbf{Metric}} & \multicolumn{4}{c}{\textbf{top-K}} \\
                \textbf{Method} & \textbf{Metric} & \textbf{Top-1}   & \textbf{Top-10}   & \textbf{Top-50}   & \textbf{Top-100}  \\  
                %\\				\cline{3-6}
				%&          & \textbf{1}   & \textbf{10}   & \textbf{50}   & \textbf{100}  \\ 
                \midrule
                
				\multicolumn{1}{c}{\multirow{2}{*}{\kw{Faiss}}}          & \kw{Prec}~(\%) &   52.0~(-44.6)  & 69.0~(-27.6)    & 73.6~(-23.0)    &    76.0~(-20.6)  \\ 
                %\cline{2-6} 
				\multicolumn{1}{c}{}                                &  \tabincell{c}{Time~(s)}    &    7.65~(3.34$\times$)  & 8.58~(3.74$\times$)    & 8.58~(3.74$\times$)     & 8.64~(3.77$\times$)     \\ 
                \midrule
                
				\multicolumn{1}{c}{\multirow{2}{*}{\Hyper}} & \kw{Prec}~(\%) & \multicolumn{4}{c}{96.6} \\ 
                %\cline{2-6} 
				\multicolumn{1}{c}{}                                & Time~(s)     & \multicolumn{4}{c}{2.29} \\ 
                \bottomrule
			\end{tabular}\par}
	\end{minipage}
%\vspace{-2ex}
\end{table}

\eat{ 
\begin{table}[t]
\vspace{-2ex}
        \setlength{\tabcolsep}{2.6pt}
	\caption{Additional datasets}\label{tab:dataset_new}
        \vspace{-2ex}
	\centering
	\scriptsize
\hspace{-0.5cm}
	\begin{tabular}{c cccccc}
		\toprule  
		\textbf{Dataset}      & \textbf{Domain}  & \textbf{\#Tuples } & \textbf{Max \#Pairs} & \textbf{\#GT Pairs} & \textbf{\#Attrs} & \textbf{\#Rules} \\ 
		\midrule
        \kw{TPCH} &synthetic     &     4M  & $1.6\times 10^{13}$    &       \#       &     8  &30 \eat{&512}\\ 
		$\kw{Songs_{sub}}$		 &     music    &     50,000     &          $\approx 2.5 \times 10^{11}$   &    \# & 8& 10\\ 
        \revise{\kw{TFACC_{large}} }&    traffic     &  36M   & $1.3\times 10^{15}$   &       \# &  16 &50 \\
		\bottomrule
	\end{tabular}	
\vspace{-6ex}
\end{table}
}

\stitle{Varying $n_t$.}
In Figures~\ref{exp:appendix}(a)-(b), we tested the impact of interval size $n_t$ on \Hyper and $\Hyper_\kw{noHO}$, that disables all hardware-level optimizations (Section~\ref{sec-exec-model}), varying $n_t$ from 32 to 512. As shown there, on \kw{TFACC},
\Hyper achieves the best performance when the interval size is 256, striking a balance between task granularity and parallelism.
\Hyper runs up to 3.1$\times$ faster than $\Hyper_\kw{noHO}$,
 verifying the usefulness of hardware optimizations on GPUs~(Section~\ref{sec-exec-model}). 
 \reviseX{The results on \kw{IMDB} are consistent.}
 \looseness=-1

\reviseS{ 
\stitle{Breakdown.}
\reviseY{We break down the time of \Hyper on  \kw{TFACC} into 4 parts in Figure~\ref{exp:move}(a):}
(1) I/O, which loads data from disk to host memory;
(2) data partition, which partitions data;
(3) plan generation, which constructs the execution plan;
(4) computation, that transfers data from the host to devices and computes matches.
As shown there, plan generation (the bottom red line) is fast, %\eg less than 0.5s; 
and
GPU operations do not dominate, consistent with findings in~\cite{GPU-Accelerated-Subgraph-Enumeration}.
\looseness=-1

\stitle{Asynchronous vs. synchronous.}
The (asynchronous) pipelined architecture (Section~\ref{sec-overview}) plays a pivotal role in \Hyper.
To justify this, we compared $\Hyper$ with $\Hyper_\kw{sync}$,
a variant without this architecture, \ie $\Hyper_\kw{sync}$ initiates the next task after the prior one is fully submitted to devices, on a synthetic dataset \kw{TPCH} generated using TPCH dbgen~\cite{TPCH} in Figure~\ref{exp:move}(b).
%Fixing $m=$ 512 with 8 GPUs. 
%Unlike $Hyper$, 
%where the scheduler of $\Hyper_\kw{sync}$ initiates the next task only after confirming that the prior task has been fully submitted to the device—effectively disabling pipelined parallelism manually.
%We varied the scale factor of both \kw{TPCH} and \kw{TFACC} from 15\% to 100\%.
%As shown there,
$\Hyper$ is %on average 3.1$\times$ 
at least 2.1$\times$ faster than $\Hyper_\kw{sync}$, due to the synchronization cost.
%since the communication %between devices and hosts 
%in $\Hyper_\kw{sync}$ is costly.
In contrast,
by asynchronously overlapping the execution at devices and the data transfer %between devices and hosts 
in \Hyper,
we reduce both the idle time and the unnecessary waiting. 
%This justifies the effectiveness of our asynchronous pipelined architecture.
%\looseness=-1

}

\begin{figure}[t]
%\vspace{-1ex}
        %%%%%%%%%%%%%%%%%%%%%%%%%%%
	% Unified legends.
	%%%%%%%%%%%%%%%%%%%%%%%%%%%
	%%%%%%%%%%%%%%%%%%%%%%%%%%%
	% Figure ROW1: COL1
	\subcaptionbox{
		\kw{TFACC}: Time breakdown
	}{
       \includegraphics[width=0.23\textwidth]{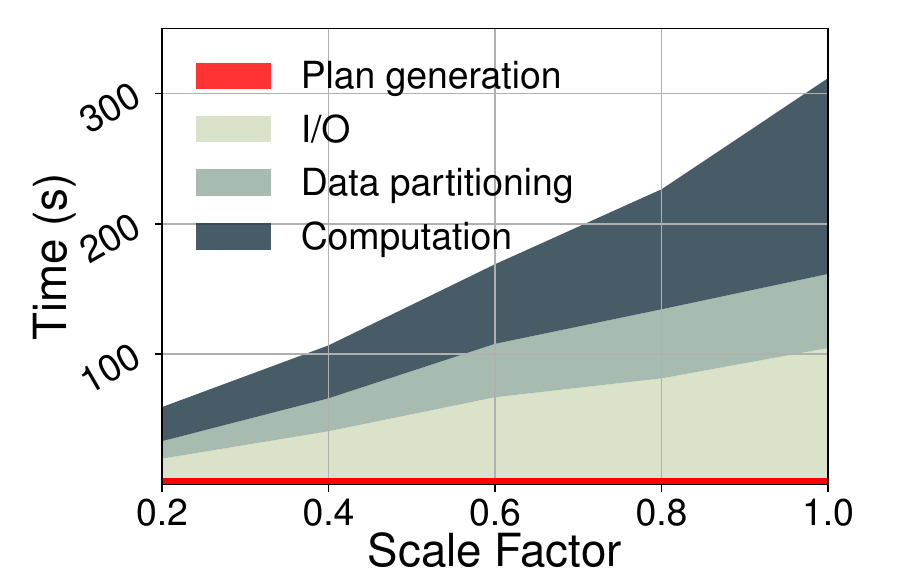}
	}
    % Figure ROW1: COL2
    \hspace{-4mm} 
	\subcaptionbox{
		\kw{TPCH}: Async. vs sync.
	}{
		\includegraphics[width=0.23\textwidth]{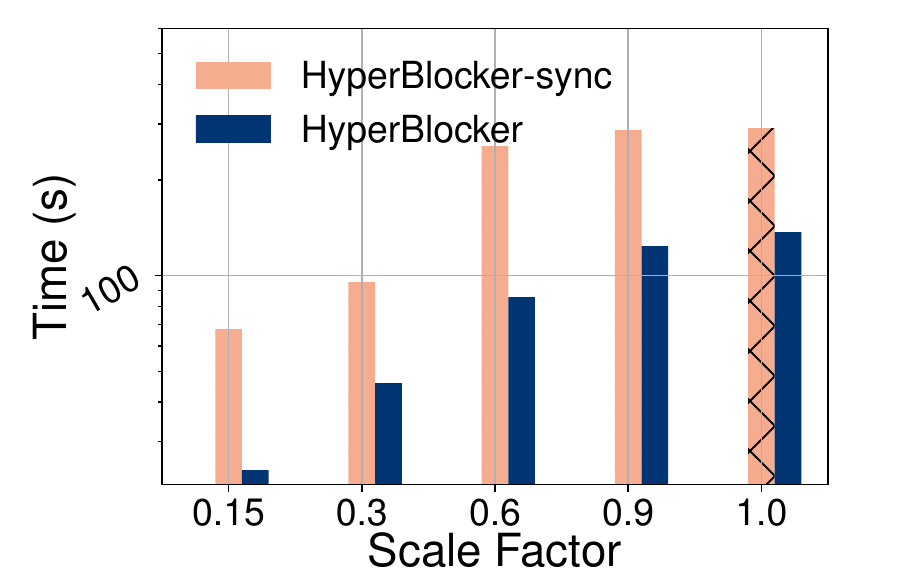}
	}
 \vspace{-3ex}
 \caption{\reviseS{Efficiency analysis} }\label{exp:move}
  \vspace{-3ex}
\end{figure}

 \reviseX{
\stitle{Experiments with more datasets.}
Figures~\ref{exp:appendix}(c)-(n) report more experimental results that are not reported in
Section~\ref{sec-expt}, due to the space limit.
These experiments were conducted under the same settings as their counter part in Section~\ref{sec-expt},  using different datasets. 
The trends are consistent and thus, the detailed analysis is omitted.

\eat{The purpose of this analysis is to validate the robustness and generalizability of our findings. 
We follow the same experimental setup and methodologies as described in the main body to ensure consistency and comparability. Detailed results are provided in Figure~\ref{exp:appendix}(f)-(l) to offer a view of how the alternative dataset impacts the experiment outcomes. }
}

\reviseX{
\stitle{Skewness on partitions.}
Figure~\ref{exp:appendix}(o)  reports
%the execution times across partitions 
%to understand the impact of partition skew on performance.
%In Figure~\ref{exp:appendix}(d),  we specifically measured 
the maximum and minimum execution times over all partitions 
using the default numbers of partitions (Table~\ref{tab:dataset}).
%to  the range of performance under skewed data conditions. The partition number is shown in Table~\ref{tab:dataset}.
As shown there, workloads can be imbalanced due to skewed execution times of partitions,
\eg the minimum execution time of a partition on \kw{Songs} is 0.01s, as opposed to 11.91s for the maximum one,
leading to performance degradation. 
The reason for the skewed execution times are twofold:
there can be skewness in the sizes of partitions and moreover,
%\eg for \kw{Songs} the maximum partition has 60k tuples, as opposed to 35 tuples for the minimum one. 
the complexity/execution depends on the underlying data,
\eg partitions containing long texts typically require more time compared to those with short texts.
To address this,
\Hyper not only adopts a collaborative approach integrating effective
partitioning and scheduling (Section~\ref{subsec:GPUs}),
but also advocates asynchronous processing (see Figure~\ref{exp:scalablity}(d)),
to improve resource utilization and overall throughput.}
%Necessitate strategies for more balanced data partitioning to achieve efficient processing times. Beside the data partition, 
%asynchronous processing is one way to alleviate load imbalance.
%As shown in Figure~\ref{fig:breakdown_sync_vs_async}, asynchronous processing, by handling smaller partitions concurrently, ensures more efficient utilization of resources and improves the overall throughput of the system.
%\looseness=-1

%\looseness=-1

\reviseX{
\stitle{Time comparison for computing the exact vs. estimated evaluation cost.} We compared the time for computing the exact and estimated evaluation costs,
denoted by $\kw{cost}(p, D)$ and $\hat{\kw{cost}}(p,D)$, respectively, in Figure~\ref{exp:appendix}(p).
Here $\kw{cost}(p, D)$ is computed by summing up the actual times for evaluating a predicate $p$ overall tuple pairs in $D$,
while $\hat{\kw{cost}}(p, D)$ is computed by replacing the actual times by the inference times of the shallow model $\mathcal{N}$.
We compute $\kw{cost}(p, D)$ and $\hat{\kw{cost}}(p, D)$ by considering all predicates that appeared in the default rule set $\Delta$ and report the average computational time per predicate.
%where reports the exact evaluation cost of the most complex predicates and the average exact evaluation cost on \kw{DBLP}-\kw{ACM}, \kw{DBLP}-\kw{Songs}, \kw{Songs}, and \kw{NCV}, respectively. 
\looseness=-1

As shown there, 
computing the estimated evaluation cost is much faster than computing the exact evaluation cost,
\eg on
\kw{NCV},
it only takes 0.008s to compute $\hat{\kw{cost}}(p, D)$ on average,
as opposed to 104.3s for $\kw{cost}(p, D)$.
Given the closeness of predicate orderings derived from both $\kw{cost}(p, D)$ and $\hat{\kw{cost}}(p, D)$ \reviseC{(see Figure~\ref{exp:scalablity}(f)),}
we justify the necessity of the use of $\mathcal{N}$ to achieve speedup.
\looseness=-1

\eat{ 
\begin{table}[t]
\caption{Time comparison (s) of exact vs. estimated costs}\label{tab:N}
\vspace{-2ex}
\setlength{\tabcolsep}{5pt}
\centering
\scriptsize
\begin{tabular}{ccccc}
\toprule
                     &                        \eat{&} \textbf{DBLP-ACM} & \textbf{DBLP-Scholar} & \textbf{Songs} & \textbf{NCV} \\

\midrule                
\textbf{Time for exact cost $\kw{cost}(p, D)$}               %& Max. & 1.4              & 195.1                & 77.8            & 195.1          \\
\eat{& Avg.}           & 0.8               & 9.3                   & 26.2            & 104.3          \\
\midrule
\textbf{Time for estimated cost $\hat{\kw{cost}}(p, D)$}   \eat{& Avg.} & 0.007               & 0.008                   &     0.009     &    0.008      \\
%\multicolumn{1}{l}{} & Avg.           & tbf               & tbf                   & tbf            & tbf \\
\bottomrule
\end{tabular}
\vspace{-3ex}
\end{table}
}

\begin{figure*}[t]
\vspace{-1ex}
        %%%%%%%%%%%%%%%%%%%%%%%%%%%
	% Unified legends.
	%%%%%%%%%%%%%%%%%%%%%%%%%%%
	%%%%%%%%%%%%%%%%%%%%%%%%%%%
	% Figure ROW1: COL1
	\subcaptionbox{
		\revise{\kw{IMDB}: Varying $n_t$}% and \#GPUs
	}{
        \includegraphics[width=0.24\textwidth]{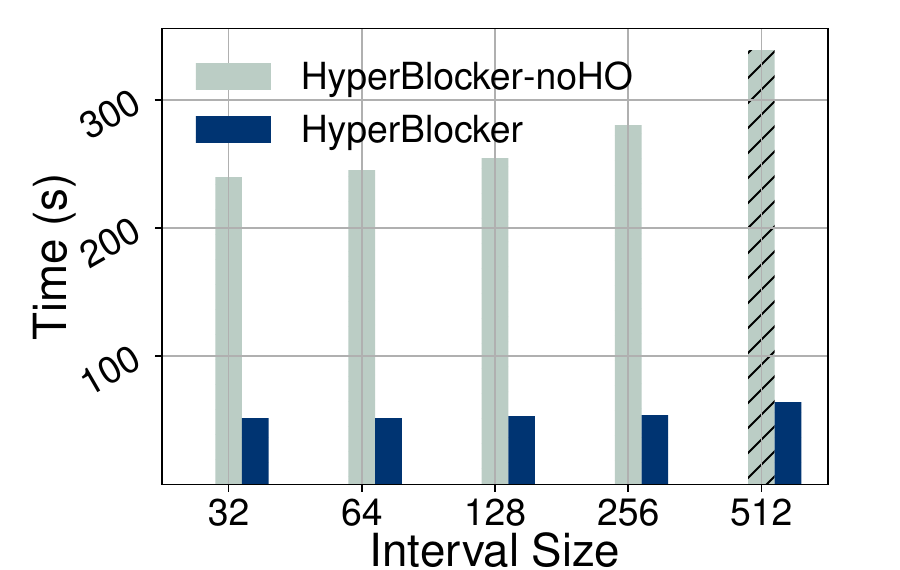}
	}
    % Figure ROW1: COL2
    \hspace{-4mm} 
	\subcaptionbox{
		\kw{TFACC}: Varying $n_t$
	}{
		\includegraphics[width=0.24\textwidth]{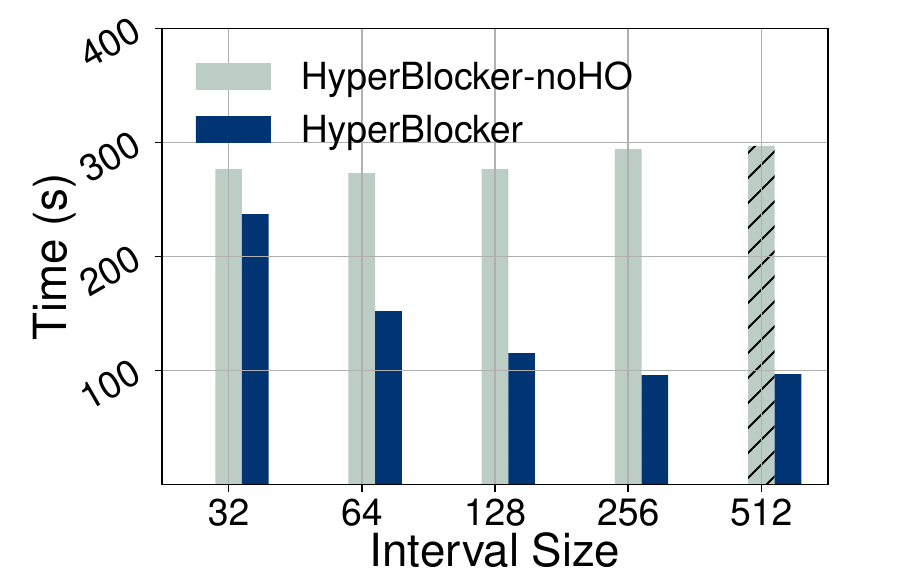}
	}
	\hspace{-4mm} 
    % Figure ROW1: COL2
        \subcaptionbox{
		\kw{DBLP}-\kw{ACM}: Impact of $m$
	}{
		\includegraphics[width=0.24\textwidth]{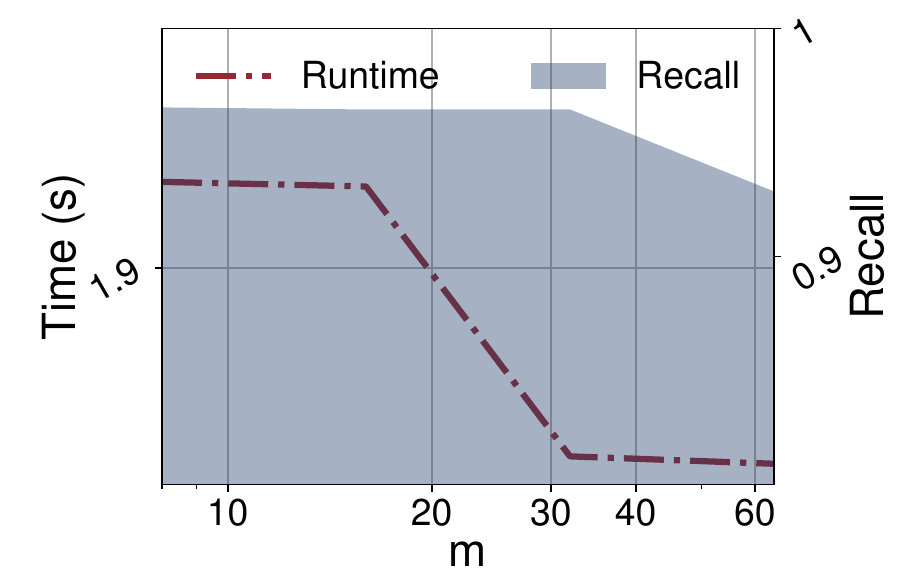}
	}   
    \hspace{-4mm}
    % Figure ROW1: COL4
        \subcaptionbox{
		\kw{Songs}: Impact of $m$
	}{
		\includegraphics[width=0.24\textwidth]{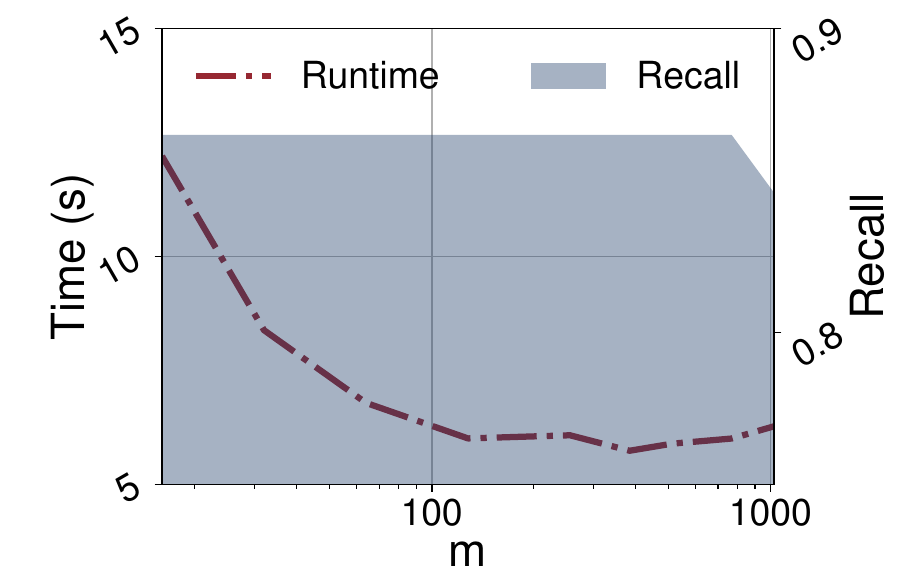}
	}

    % Figure ROW2: COL1
        \subcaptionbox{
		\kw{TPCH}: Varying \#GPUs
	}{
        \includegraphics[width=0.24\textwidth]{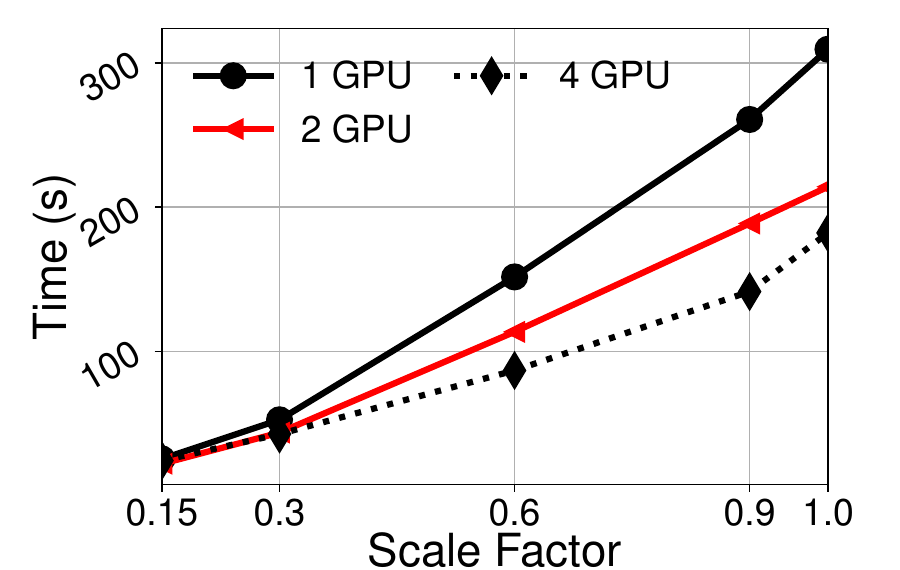}\vspace{-1.5ex}
	} 	     
 	\hspace{-4mm}
    % Figure ROW2: COL2
    \subcaptionbox{
		\kw{TFACC}: Varying \#GPUs
	}{
        \includegraphics[width=0.24\textwidth]{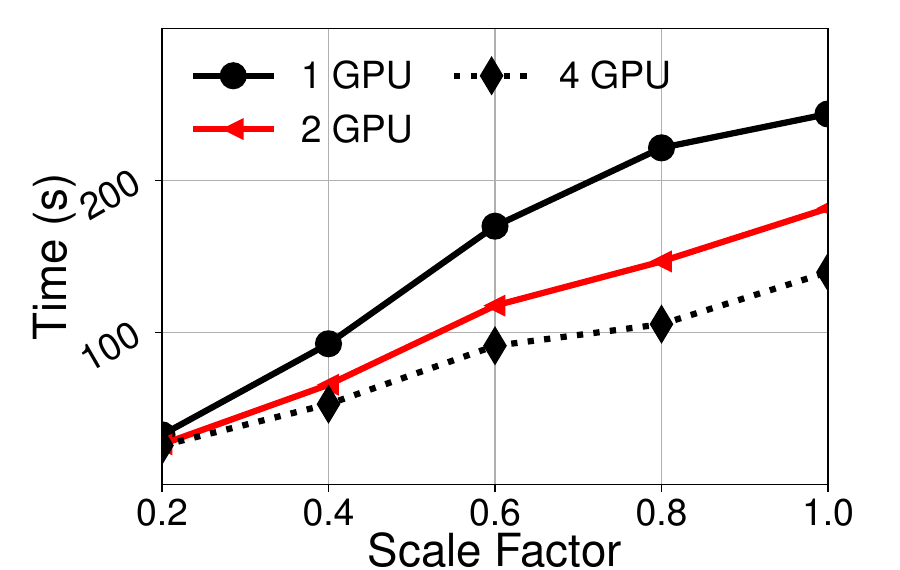}\vspace{-1.5ex}
	} 
    \hspace{-4mm}
    % Figure ROW2: COL3
    \subcaptionbox{
		\kw{TFACC}: Async vs sync.
	}{
		\includegraphics[width=0.24\textwidth]{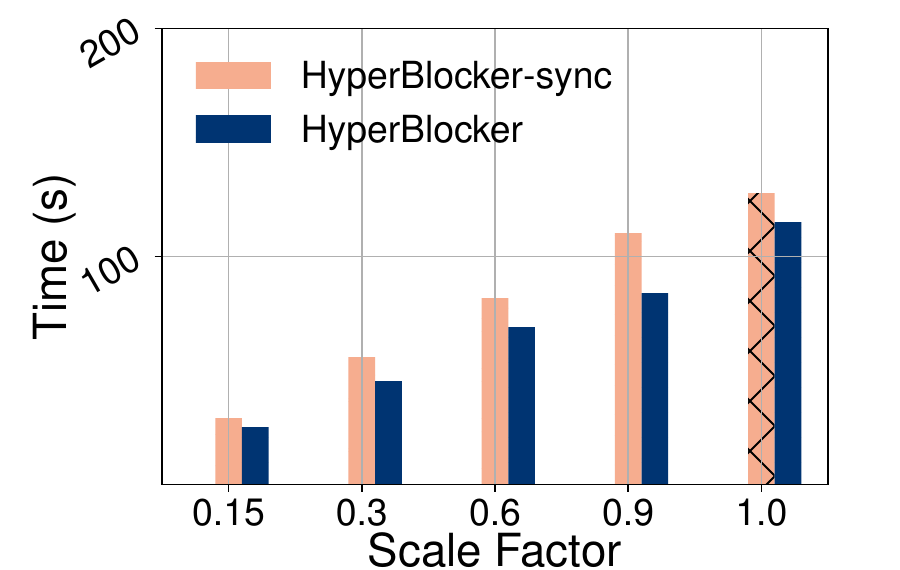}\vspace{-1.5ex}
	}     
 	\hspace{-4mm}
    % Figure ROW2: COL4
        \subcaptionbox{
		\kw{NVC}: Async vs sync.
	}{
		\includegraphics[width=0.24\textwidth]{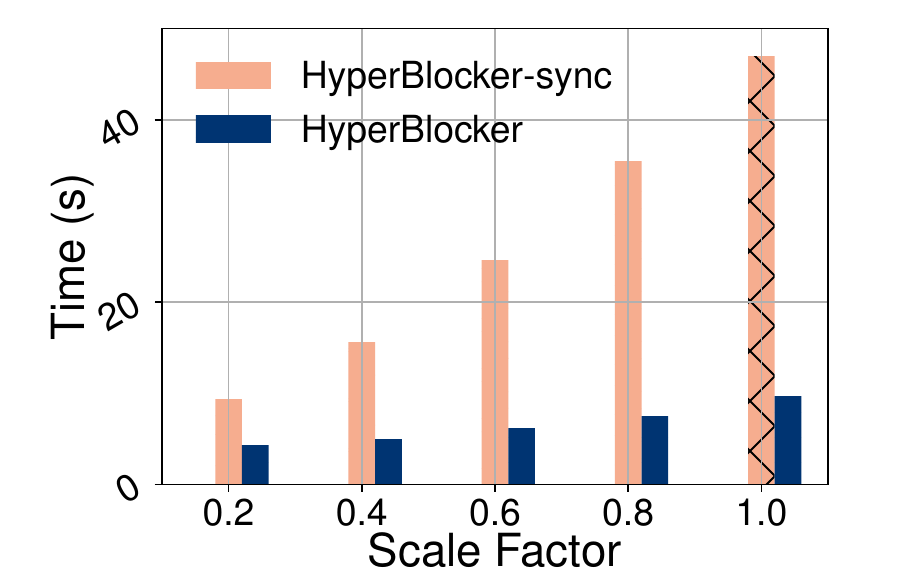}\vspace{-1.5ex}
	}

    % Figure ROW3: COL1
    \subcaptionbox{
		\revise{\kw{TFACC}: impact of scheculers}
	}{
		\includegraphics[width=0.24\textwidth]{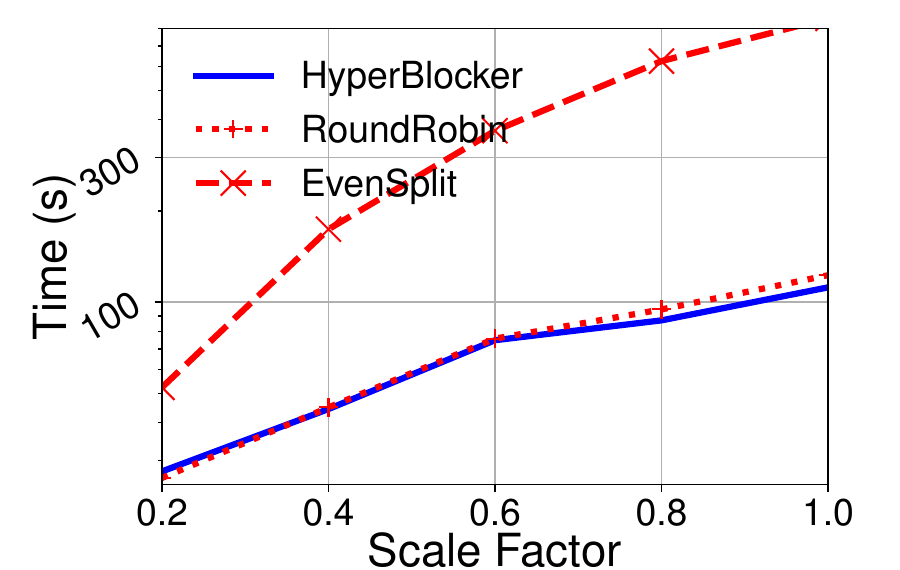}\vspace{-1.5ex}
	}
    \hspace{-4mm} 
    % Figure ROW3: COL2
        \subcaptionbox{
		\revise{\kw{IMDB}: Varying $|\varphi|$}% and \#GPUs
	}{
        \includegraphics[width=0.24\textwidth]{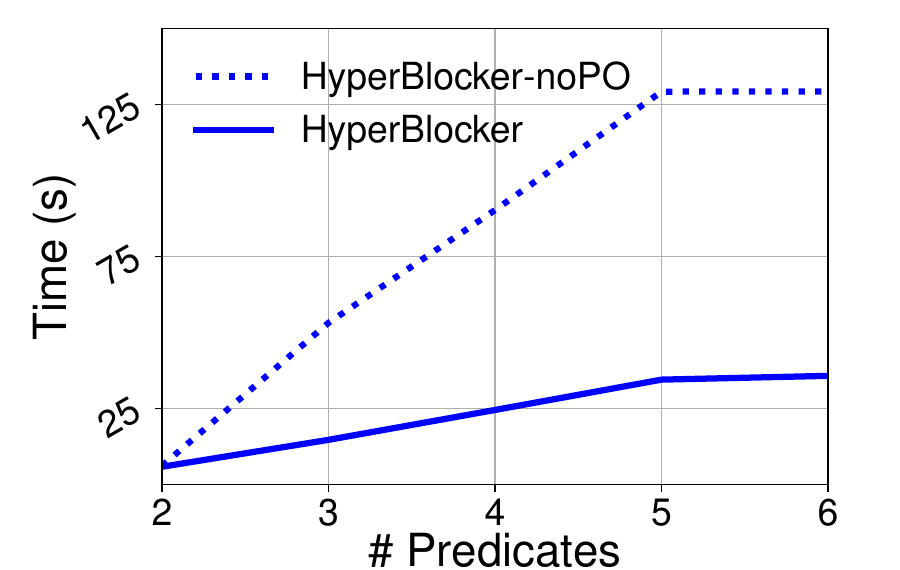}\vspace{-1.5ex}
	}
     \hspace{-4mm} 
    % Figure ROW3: COL3
        \subcaptionbox{
		\kw{Songs}: Varying $|\varphi|$}% and \#GPUs
	{
        \includegraphics[width=0.24\textwidth]{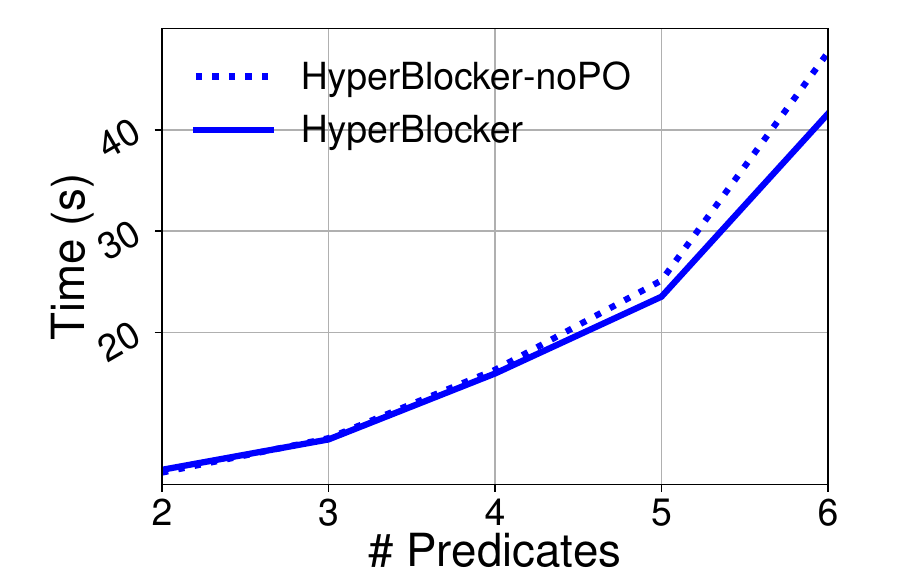}\vspace{-1.5ex}
	}
     % Figure ROW3: COL4
    \hspace{-4mm} 
	\subcaptionbox{
		\kw{IMDB}: Varying $|\Delta|$
	}{
		\includegraphics[width=0.24\textwidth]{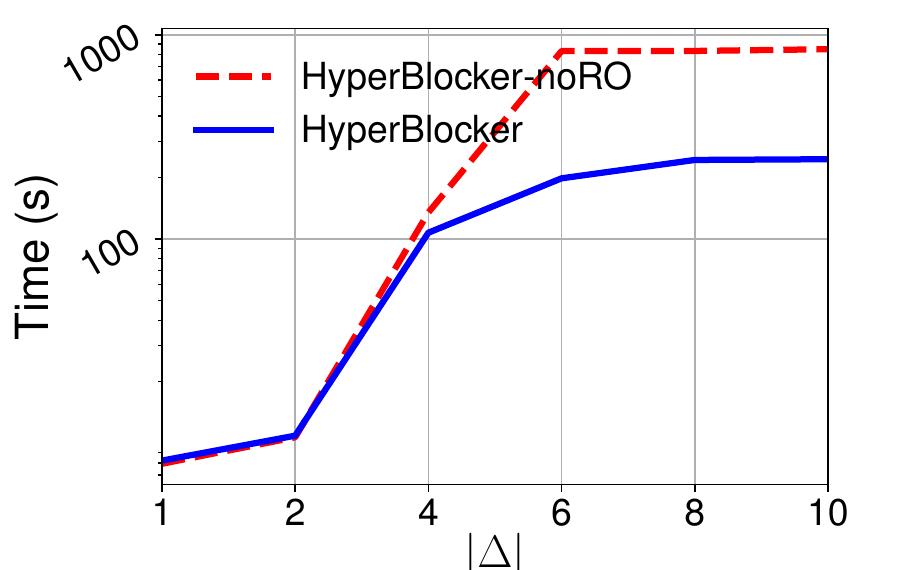}\vspace{-1.5ex}
	}
 
    % Figure ROW4: COL1
    \subcaptionbox{
	\kw{Songs}: Varying noise\%}
	{
		\includegraphics[width=0.24\textwidth]{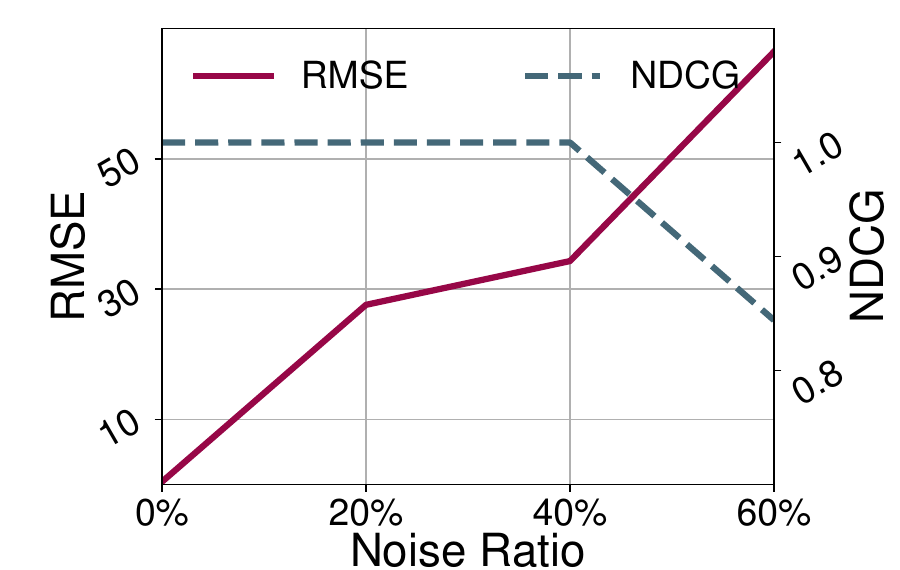}\vspace{-1.5ex}
	}
    \hspace{-4mm} 
    % Figure ROW4: COL2
    \subcaptionbox{
	\kw{IMDB}: Varying noise\%}
	{
		\includegraphics[width=0.24\textwidth]{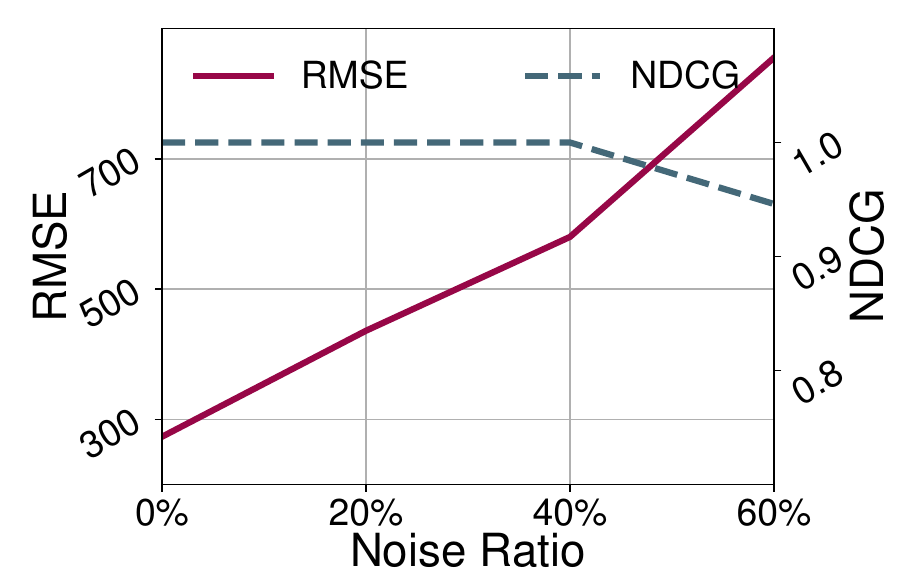}\vspace{-1.5ex}
	}
     \hspace{-4mm} 
    % Figure ROW4: COL3
    \subcaptionbox{
		Skewness statistic}% and \#GPUs
	{
        \includegraphics[width=0.24\textwidth]{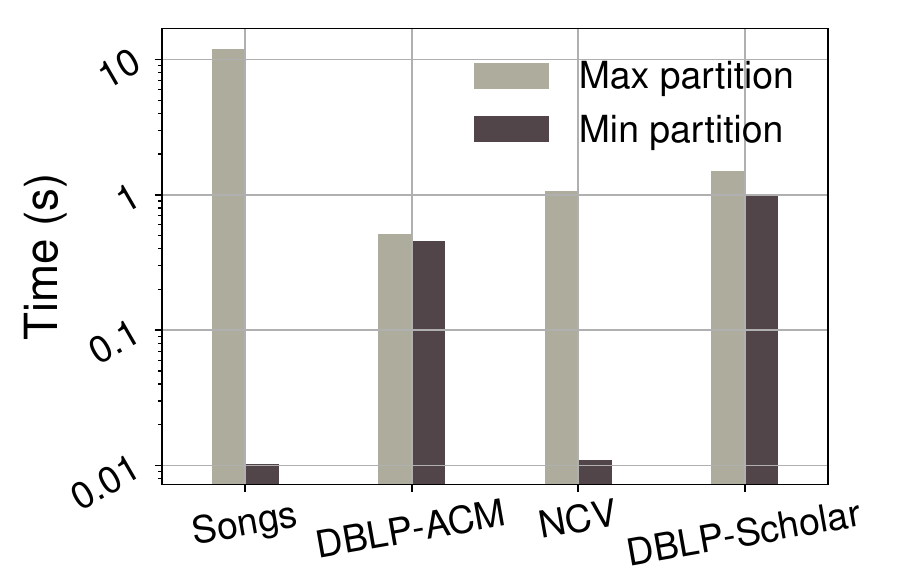}\vspace{-1.5ex}
	}
     % Figure ROW4: COL4
    \hspace{-4mm} 
	\subcaptionbox{
		Exact cost vs. Estimated cost
	}{
		\includegraphics[width=0.24\textwidth]{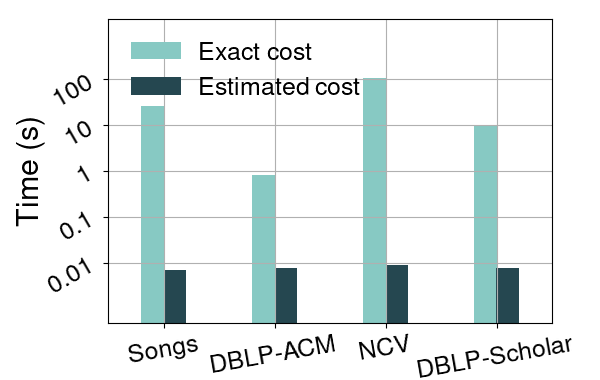}\vspace{-1.5ex}
	}
   
    \vspace{-2ex}
    \caption{Additional experimental results} \label{exp:appendix}
    \vspace{-2ex}
\end{figure*}

\eat{ 
Figure~\ref{exp:overall}(k) illustrates the sensitivity of $\mathcal{N}$  to training data noise and shows the tolerance of \kw{EPG}~(Section~\ref{sec-plan}) to changes in data distribution.  Different levels of gaussian noise (ranging from 20\% to 60\%) were introduced into the training data to simulate changes in data distribution. On \kw{DBLP}-\kw{ACM}, the relationship between noise ratio and performance metrics (NDCG~\cite{NDCG} and RMSE) was reported where NDCG compares the generated order to an ideal matching order of rules. 
As shown there, 
(1) with increasing noise, the RMSE of $\mathcal{N}$ becomes larger, as expected. (2) The \kw{EPG} shows high tolerance to distribution changes, with less steep declines in NDCG.
}

\stitle{Case study on predicate orderings.}
Recall that in \reviseC{Figure~\ref{exp:scalablity}(f),}
we report the performance of $\mathcal{N}$ 
by varying the noise ratio $\beta \%$,
and we show that with more noises,
$\N$ is less accurate, as expected.
However,
one may notice that
even if the predictions of $\mathcal{N}$ have a larger RMSE,
it does not necessarily affect the resulting predicate orderings,
as long as the relative orders of predicates are the same.

To show this, below we report a case study on the resulting predicate orderings under different noise ratios on \kw{DBLP}-\kw{ACM} using four predicates,
namely  $p_1: t.\kw{year} = s.\kw{year}$, $p_2:  t.\kw{authors} \approx_\kw{ED} s.\kw{authors}$, $p_3: t.\kw{venue} \approx_\kw{JD} s.\kw{venue}$,  and $p_4:  t.\kw{title} \approx_\kw{JD} s.\kw{title}$.
When $\beta \% = 0\%$, 
the predicate ordering estimated via $\N$ is 
O1: $p_1, p_2, p_3, p_4$,
which is the same as the ground truth ordering derived from the actual costs.
This ordering is unchanged even if we inject 20\% noises to the training data of $\N$.
However,
when we injected 40\% noises, the predicate ordering is changed to
O2: $p_1, p_3, p_2, p_4$,
\ie only the relative order of $p_2$ and $p_3$ is swapped.
When we further increased the noise ratio to 60\%,
the predicate ordering becomes more messy,
\ie O3: $p_2, p_3, p_1, p_4$.

\eat{
we list the generated rules at 40\% and 60\% noise levels, comparing them to the ideal matching rule, denoted as $\varphi_{40\%}$, $\varphi_{60\%}$, and $\varphi_\kw{Ideal}$ respectively.
\mbi
\item $\varphi_\kw{Ideal}:  t.\kw{year} = s.\kw{year}  \land t.\kw{venue} \approx_\kw{JD} s.\kw{venue} \land t.\kw{authors} \approx_\kw{ED} s.\kw{authors} \allowbreak \land t.\kw{title} \approx_\kw{JD} s.\kw{title} \to t.\kw{eid} = s.\kw{eid}$
\item $\varphi_{40\%}:  t.\kw{year} = s.\kw{year}  \land t.\kw{authors} \approx_\kw{JD} s.\kw{authors} \land t.\kw{venue} \approx_\kw{JD} s.\kw{venue} \allowbreak \land t.\kw{title} \approx_\kw{JD} s.\kw{title} \to t.\kw{eid} = s.\kw{eid}$
\item $\varphi_{60\%}: t.\kw{authors} \approx_\kw{JD} s.\kw{authors} \land t.\kw{venue} \approx_\kw{JD} s.\kw{venue} \land t.\kw{year} = s.\kw{year}   \allowbreak \land t.\kw{title} \approx_\kw{JD} s.\kw{title} \to t.\kw{eid} = s.\kw{eid}$
\mei
When the data distribution changes to 40\%, it simply switches positions of $t.\kw{venue} \approx_\kw{JD} s.\kw{venue}$ and $t.\kw{authors} \approx_\kw{JD} s.\kw{authors}$.
This justify  robustness of \kw{EPG}.}

\eat{ 
\stitle{Runtime statistics analysis.}
Table~\ref{tab:runtime} reports \eat{various}
runtime statistics on \kw{TFACC} compared with variants of \Hyper: $\Hyper_\kw{noSeq}$, $\Hyper_\kw{noPSW}$, $\Hyper_\kw{noStealing}$.

As shown, \Hyper has significantly better warp utility than its variants, achieving an average of 28.21 active threads per warp and the lowest wait stalls. This is because (1) while branch divergence is sometimes unavoidable, a recursive implementation further increases thread stalls, thus harming performance; (2) without PSW, the workload assignment is relatively skewed, resulting in fewer active threads per warp; (3) \Hyper supports task stealing from heavily burdened threads, thus reducing thread stalls. The result justifies our hardware-aware optimizations.
}

\eat{ 
\begin{table}[h]
\caption{Runtime statistics for $\Hyper_\kw{noSeq}$, $\Hyper_\kw{noPSW}$, $\Hyper_\kw{noStealing}$, and \Hyper.}\label{tab:runtime}
\setlength{\tabcolsep}{5pt}
\centering
\scriptsize
\begin{tabular}{clccc}
\toprule
                                      & \textbf{noSeq} & \textbf{noPSW} & \textbf{noStealing} & \textbf{\Hyper} \\
                                      \midrule
\textbf{\tabincell{c}{Avg. active threads per warp}} & 14.45 & 25.59 & 27.62 & 28.21\\
\textbf{\tabincell{c}{Circles spent in wait stalls}} & 4.25 & 13.79 & 4.11 & 4.07\\
\textbf{\tabincell{c}{Branch efficiency (\%)}} & 89.9 & 96.3 & 96.2 & 96.4\\
%\textbf{\tabincell{c}{Avg. Divergent Branches}} & 8414 & 8447 & 8414 & 8414\\
\bottomrule
\end{tabular}
\end{table}
}
}

\eat{
\begin{figure*}[t]
%\vspace{-3ex}
	\centering
	\includegraphics[width=1\linewidth]{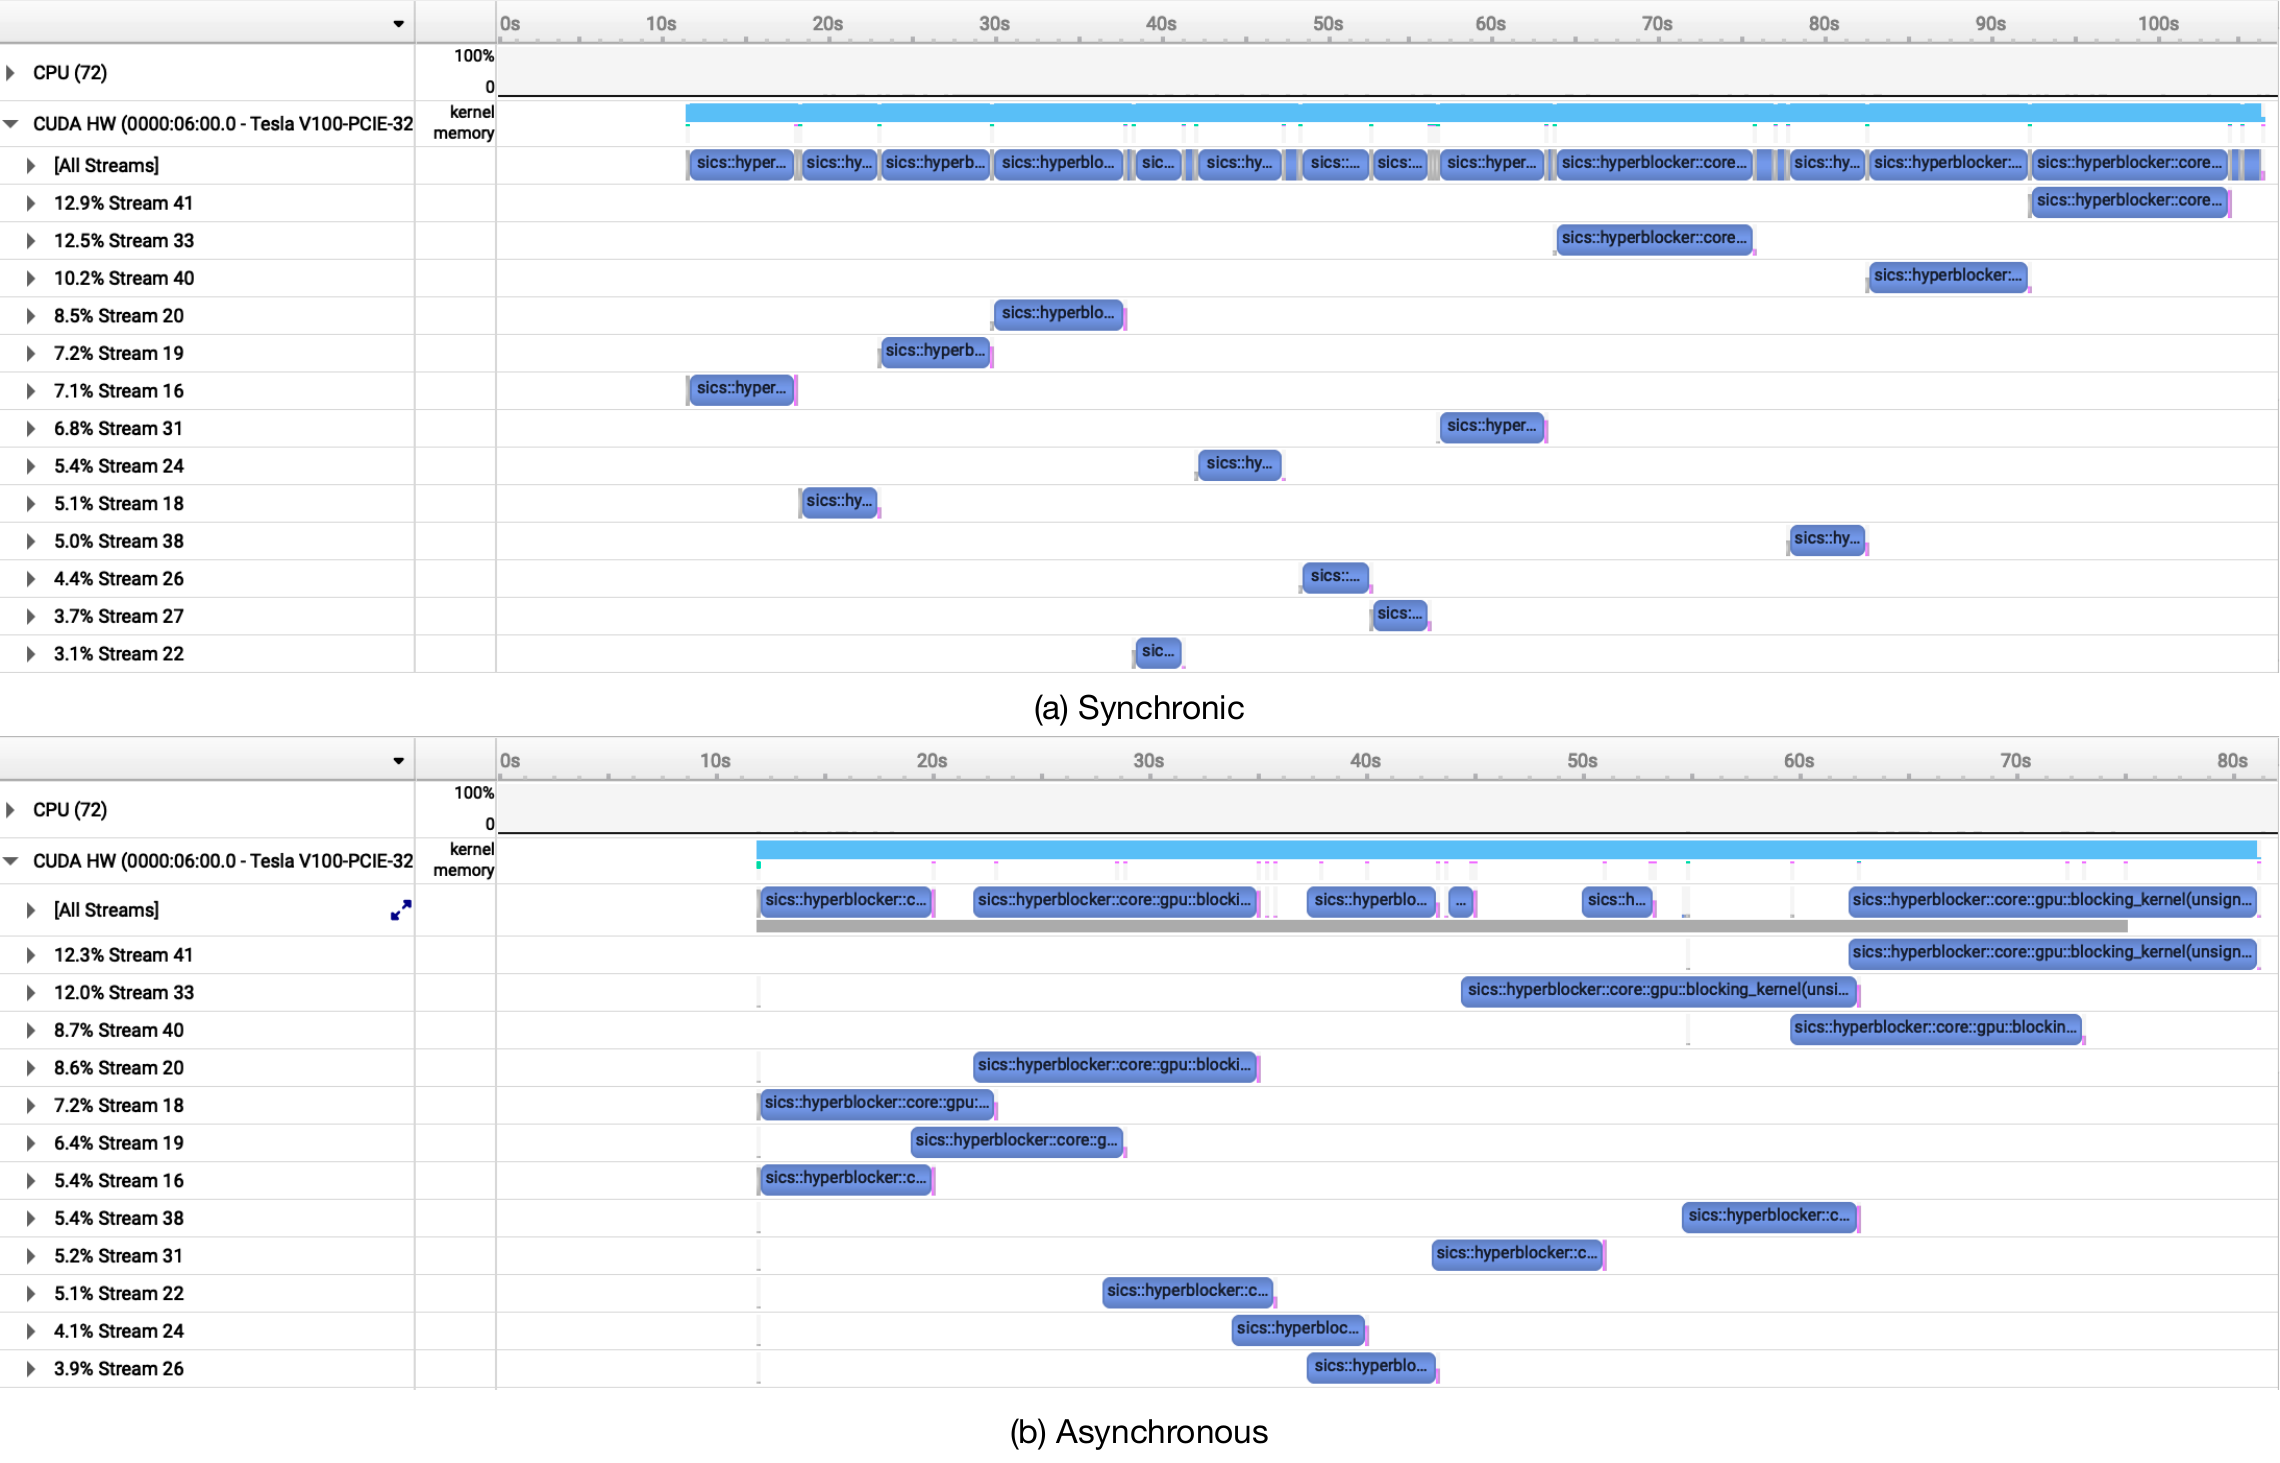}
 \vspace{-4ex} 
	\caption{Songs: elapsed time of each stream.}
	\label{fig:breakdown_sync_vs_async}
\vspace{-3ex} 
\end{figure*} 
}

\stitle{Case study on single vs. multi-execution plans.}
As remarked in Section~\ref{sec-plan},
plan generation in \Hyper can be regarded as a pre-processing step for blocking,
\ie
once a plan is generated,
it is applied in \emph{all} partitions of $D$.
However,
it is also possible to group tuples into different partitions/clusters and generate 
an execution tree for each partition/cluster.
%We are aware that there is a change in data distribution after partitioning. A unique execution tree for all partitions might not be optimal. To determine if multiple execution trees are needed for optimal performance, 
We report a carefully designed case study,
comparing two methods: 
(1) $\Hyper_\kw{same}$ that uses the same execution plan for all partitions and 
(2) $\Hyper_\kw{mult}$ that generates a different execution plan for each partition.
%We use \kw{DBLP}-\kw{Scholar}, which contains 34,790 tuples with null values in the "year" attribute. 
Here we used \kw{DBLP}-\kw{Scholar} and split it into two partitions $P_1$ and $P_2$, where $P_1$ (resp. $P_2$) contains tuples with null (resp. non-null) values on \kw{year}.
We designed two blocking rules, namely $\varphi_a$ and $\varphi_b$: \looseness=-1

\mbi
\item $\varphi_a: t.\kw{authors} \approx_\kw{JD} s.\kw{authors} \land t.\kw{title} \approx_\kw{JD} s.\kw{title} \land t.\kw{year} = s.\kw{year} \allowbreak \to t.\kw{eid} = s.\kw{eid}$; and
\mei
\mbi
\item $\varphi_b: t.\kw{year} = s.\kw{year} \land t.\kw{authors} \approx_\kw{JD} s.\kw{authors} \land t.\kw{title} \approx_\kw{JD} s.\kw{title} \allowbreak  \to t.\kw{eid} = s.\kw{eid}$.
\mei

For simplicity,
we assume each execution plan consists of exactly one rule,
leading to two execution plans, namely $\mathcal{T}_1 = \{\varphi_a\}$ and $\mathcal{T}_2 = \{\varphi_b\}$,
where the predicates in each rule are evaluated in the order they appear above (\eg $t.\kw{year} = s.\kw{year}$ is evaluated first in $\mathcal{T}_2$).
Moreover,
$\Hyper_\kw{same}$ used $\varphi_a$ for both partitions, while $\Hyper_\kw{mult}$ used $\varphi_a$ for $P_1$ and used $\varphi_a$ for $P_2$.
%and optimized execution plan $\Hyper_\kw{P_2}$ for $P_2$, respectively.
\looseness=-1

By the results, $\Hyper_\kw{mult}$ accelerates $\Hyper_\kw{same}$ by 32.7\%,
since $\Hyper_\kw{same}$ adopts a poor execution plan:
while distinct years are good indicators of mismatches and years are cheap to compare,
$\mathcal{T}_1$ compares the values on years at the end of plan.
In contrast,
by applying $\mathcal{T}_2$, that compares years first, on $P_2$,
we can quickly discard tuple pairs with distinct years 
(but this is not possible for $P_1$,
where all tuples have the same value on years).

This case study showcases that it is indeed possible to improve the overall performance  using  a different execution plan for each partition,
compared with a global execution plan for all partitions.
However, 
after conducting tests on other datasets using the general setting, 
we find that the performance gain is not remarkable. 
This is because the global execution plan generated by EPG is not as poor as $\mathcal{T}_1$
and it works sufficiently well for most partitions.
Moreover,
the effectiveness of multiple execution plans also depends on the data distributions in different partitions,
\eg in \kw{DBLP}-\kw{ACM}, the data distributions do not vary much across different partitions, so that a single execution plan suffices for reasonably good performance.
Nevertheless,
we plan to further optimize \Hyper over multiple execution plans as a promising future direction.

\begin{table}[t]
\caption{\reviseS{Time comparison (s) under different execution plans}}\label{tab:postgres}
\vspace{-2ex}
\setlength{\tabcolsep}{5pt}
\centering
\scriptsize
\begin{tabular}{ccccc}
\toprule
  \textbf{Method}           & \kw{Songs} & \kw{DBLP}-\kw{ACM} & \kw{NCV} & \kw{IMDB} \\
\midrule
\kw{PostgreSQL}   & 40.6~($3.0\times$) & 0.7~($2.3\times$) &  13.5~($2.2\times$)   &   13036.0~($449.5\times$)           \\
\kw{TupleX}   & 14.2~($1.04\times$) & 0.4~($1.3\times$) &  12.4~($2.0\times$)   &   36.1~($1.2\times$)           \\
\kw{EPG} & 13.6 & 0.3 &     6.2   &  29.0            \\
\bottomrule
\end{tabular}
\end{table}

\reviseS{
\stitle{Case analysis on the optimizers of existing DBMS.}
To investigate the effect of existing DBMS when optimizing the ordering of UDFs and dealing with {\tt OR} operations,
we tested the performance of \kw{PostgreSQL}~\cite{postgresql}, a widely adopted DBMS, on the following four SQL queries on 
the \kw{DBLP}-\kw{ACM} dataset~\cite{magellandata}, where each tuple is described by four attributes, namely \kw{title}, \kw{authors}, \kw{venue} and \kw{year}.
\mbi 
\item $\Q_1$: {\tt SELECT *  FROM \kw{DBLP}, \kw{ACM} WHERE \kw{DBLP}.\kw{title} $\approx$ \kw{ACM}.\kw{title} AND \kw{DBLP}.\kw{authors} $\approx$ \kw{ACM}.\kw{authors} AND \kw{DBLP}.\kw{year} = \kw{ACM}.\kw{year}};
\item $\Q_2$: {\tt SELECT * FROM \kw{DBLP}, \kw{ACM} WHERE \kw{DBLP}.\kw{authors} $\approx$ \kw{ACM}.\kw{authors} AND \kw{DBLP}.\kw{title} $\approx$ \kw{ACM}.\kw{title}  AND \kw{DBLP}.\kw{year} = \kw{ACM}.\kw{year}};
\item $\Q_3$: {\tt SELECT * FROM \kw{DBLP}, \kw{ACM} WHERE \kw{DBLP}.\kw{venue} $\approx$ \kw{ACM}.\kw{venue} AND \kw{DBLP}.\kw{title} $\approx$ \kw{ACM}.\kw{title}  AND \kw{DBLP}.author = \kw{ACM}.author};
\item $\Q_4$: {\tt SELECT * FROM \kw{DBLP}, \kw{ACM} WHERE \kw{DBLP}.\kw{authors} $\approx$ \kw{ACM}.\kw{authors} AND \kw{DBLP}.\kw{title} $\approx$ \kw{ACM}.\kw{title}  AND \kw{DBLP}.\kw{year} = \kw{ACM}.\kw{year} OR  \kw{DBLP}.\kw{venue} $\approx$ \kw{ACM}.\kw{venue} AND \kw{DBLP}.\kw{title} $\approx$ \kw{ACM}.\kw{title} AND  \kw{DBLP}.\kw{authors} = \kw{ACM}.\kw{authors}}.
\mei
where $\kw{DBLP}.A \approx \kw{ACM}.A$ denotes the similarity comparison on attribute $A$ (where $A \in \{\kw{title}, \kw{authors}, \kw{venue}\}$)
and it is implemented as a User Defined Function (UDF) following ~\cite{rock,preedet}.
Note that (a) $\Q_1$ and $\Q_2$ only differ in the order of two UDFs and 
(b) the condition of the {\tt WHERE} clause of $\Q_4$ can be regarded as a disjunction (\ie\  {\tt OR}) of those of 
$\Q_2$ and $\Q_3$.
They were used to evaluate the capability of the optimizer of \kw{PostgreSQL} when handling UDFs and {\tt OR}, respectively. \looseness=-1

Each query was run 10 times. The average runtime was compared.
With \kw{PostgreSQL}’s {\tt EXPLAIN} feature, we observe the following: \looseness=-1

\sstab 
(1) Even though the equality comparison (\kw{DBLP}.\kw{year} = \kw{ACM}.\kw{year}) is specified at the end of both $\Q_1$ and $\Q_2$,
\kw{PostgreSQL} optimizes the execution, by prioritizing the equality comparison, to use the hash index on \kw{year} early.
In contrast,
$\Q_2$ was consistently faster than $\Q_1$ by 20\% on average.
This is because, unlike equality comparisons, \kw{PostgreSQL} does not optimize the order of UDFs for similarity comparisons well,
\eg it evaluates similarity predicates simply in the same order as they are specified in the queries.
This leads to a performance gap when the two UDFs are not equally potent for evaluation. \looseness=-1

\sstab
(2) On average, $\Q_4$ takes 12$\times$ longer than $\Q_2$ and $\Q_3$, respectively.
This is because $\Q_4$ performs sequential scans with a nested loop, 
instead of utilizing the hash index like $\Q_2$ does.
This said, using the {\tt OR} operators can prevent the database from effectively using indexes, leading to suboptimal execution plans and poor performance.

\vspace{0.6ex}
These findings justify that existing optimizers of DMBS may struggle to handle rule-based blocking efficiently,
even though it can be implemented with a SQL query,
due to the DNF nature of blocking and the UDFs for evaluating similarity comparisons.
}

\reviseS{ 
\stitle{Execution plan of EPG vs. PostgreSQL and TupleX.}
To further evaluate the performance of EPG,
we replaced the execution plan generated by EPG in \Hyper with alternative plans generated by other systems
and report the runtime of the resulting blocking.
Specifically,
we compared the plans from the following systems:
(1) \kw{PostgreSQL}~\cite{postgresql}, a widely adopted DBMS;
we extract its execution plan using the {\tt EXPLAIN} feature.
(2) \kw{TupleX}~\cite{tuplex},
which is designed for Python-based UDFs optimization for data processing;
we format the query logic in Python and extract the plan from the log file.

As shown in Table~\ref{tab:postgres},
the execution plan generated by EPG consistently beats the one generated by \kw{PostgreSQL}  by $114\times$ (resp. \kw{TupleX} by 38.5\%) on average on all datasets.
As remarked in the previous experiments, the reasons are threefold:
(1) \kw{PostgreSQL} treats UDFs as black boxes and may mistakenly prioritize high-cost predicates, \eg
this leads to a $449.5\times$ slowdown on the \kw{IMDB} dataset.
In contrast, 
by analyzing the evaluation time and the  selectivity using the learned LSH-based method, 
EPG accurately estimates the cost-effectiveness of each predicate.
(2) EPG produces the evaluation order of predicates based on the aforementioned cost-effectiveness, while
the evaluation order of multiple UDFs in \kw{PostgreSQL} heavily depends on how the user writes them the SQLs.
Although \kw{TupleX} can reorder predicates by sampling data, it still leads to a suboptimal execution plan since its optimizations rely solely on the data/operation types, without accounting for the data distribution (\ie lack data-awareness), which can significantly affect performance.
(3) EPG evaluates rules in a DFS manner on the tree structure to cope with the disjunction logic of blocking and uses bitmaps to reuse computations as much as possible (see Section \ref{sec-plan}), whereas \kw{PostgreSQL} may require a sequential scan of all data in certain cases.
}\looseness=-1

\eat{ 
Creating an efficient execution plan for blocking remains an open problem, 
with optimizing UDFs and "OR" clauses being two key challenges. 
To illustrate the benefits of EPG, we evaluated the execution time under different plans. 
We used PostgreSQL's plan extracted via its EXPLAIN feature and the plan of \kw{TupleX}~\cite{tuplex}, 
designed for Python-based UDFs optimization for data processing, 
by writing the query logic in Python and extracting the plan from the log file.

All execution plans were then executed using the \Hyper model. 
The results showed that EPG's execution plan consistently outperformed PostgreSQL's by $114\times$ on average 
and \kw{TupleX} by 26\%.

The reasons are threefold:
(1) By analyzing predicates' filtering ability via an LSH-based method and potential execution costs through a learned model, EPG provides a more accurate prediction of computation costs for an execution plan. In contrast, PostgreSQL's handling of multiple UDFs heavily depends on how the user writes the SQL, and although \kw{TupleX} can reorder predicates by sampling data and analyzing the execution tree, it remains suboptimal.
(2) EPG's execution plan can shortcut computations across rules using a tree structure and bitmap index (see Section \ref{sec-plan}), whereas PostgreSQL's plan requires a sequential scan of all data.
(3) PostgreSQL treats UDFs as black boxes and might mistakenly prioritize high-cost predicates. For example, prioritizing predicates with high cost on the \kw{IMDB} dataset led to a $449\times$ higher cost than EPG.

These differences in execution plans explain EPG's performance advantage over PostgreSQL and \kw{TupleX}.
}
